# Supplementary material for: A fast and spectrally convergent algorithm for rational-order fractional integral and differential equations
Source: arXiv:1611.08028 source file (2017-12-01)
Supplement: Supplementary file 1 [file appendixB.tex]

Consider the following example:
$$u_t = D^{3/2} u$$
with $u(t,1) = 0$, which one would  expect to behave half way between a transport and a diffusion equation.   Applying the Trapezoidal rule with $h = ?$ produces Figure ?, which looks reasonable.  However, the condition number blows up as $h \rightarrow 0$.  Understanding the root of this issue and how it might be overcome is an ongoing project.
